# Supplementary material for: Montessori-Instruct: Generate Influential Training Data Tailored for Student Learning
Source: arXiv:2410.14208 source file (2024-10-18)
Supplement: Supplementary file 1 [file algorithm.tex]

\begin{algorithm}
    \caption{Training Language Models to Generate Influential Synthetic Training Data.\zichun{This is too long and not very informative (like the training part is not neccessary). We only need to elaborate the one-step probing \& preference dataset creation in our main text. Maybe put it in the Appendix?}}
    \label{alg:cap}
    \begin{algorithmic}
    \Require Seed pool $\mathcal{D}_S$, task-related validation dataset $\mathcal{D}_T$, warmup dataset $\mathcal{D}_{warmup}$, selection dataset $\mathcal{D}_{selection}$, loss dataset $\mathcal{D}_{loss}$, preference dataset $\mathcal{D}_{pre}$, data synthesis model $\mathcal{M}$, task model $m$, warmup steps $T_W$, total training steps $T$, DPO training algorithm $\mathcal{A}_D$, SFT training algorithm $\mathcal{A}_S$
    \Ensure $\mathcal{D}_{warmup}$, $\mathcal{D}_{selection}$, $\mathcal{D}_{loss}$ and $\mathcal{D}_{pre}$ are all empty.
    \vspace{0.5mm}
    \State $\mathcal{D}_{warmup} \gets  \mathcal{M}_t(\mathcal{D}_S)$ \Comment{Warmup Stage}
        \For{$t \gets 1 \text{ to } T_W$}    
            \State Sample a batch $B_t$ from $\mathcal{D}_{warmup}$
            \State $m \gets \mathcal{A}_S(m, B_t)$
        \EndFor
    \State $\mathcal{D}_{selection} \gets \mathcal{M}_t(\mathcal{D}_S)$ \Comment{Collect one-step-train loss}
        \For{$i \gets 1 \text{ to } |\mathcal{D}_{selection}|$} 
            \State Select one data $(p_i, x_i^j, y_i^j)$ from $\mathcal{D}_{selection}$
            \State $m_{copy} \gets m$
            \State $m^{ij}_{copy} \gets \mathcal{A}_S(m_{copy}, (x_i^j, y_i^j)))$
            \State $I_i^j \gets l(m^{ij}_{copy}, \mathcal{D}_T) - l(m_{copy}, \mathcal{D}_T)$
            \State add $(p_i, x_i^j, y_i^j, I_i^j)$ to $\mathcal{D}_{loss}$
        \EndFor
    \For {$i \gets 1 \text { to } |\mathcal{D}_{loss}|$} \Comment{Create Preference Dataset}
        \For {$k \gets i+1 \text { to } |\mathcal{D}_{loss}|$}
            \If {$p_i = p_k \text{ AND } (I_i < 0 < I_k \text{ OR } I_k < 0 < I_i)$}
            \State add $(p_i, x_i, x_k)$ to $\mathcal{D}_{pre}$
            \EndIf
        \EndFor
    \EndFor
    \State $\mathcal{M}^{'} \gets \mathcal{A}_D(\mathcal{M}, \mathcal{D}_{pre})$ \Comment{Update Data Synthesis Model}
    \State $\mathcal{D} \gets \mathcal{M}^{'}(\mathcal{D}_S)$
        \For{$t \gets 1 \text{ to } T$}    \Comment{Train the task model}
            \State Sample a batch $B_t$ from $\mathcal{D}$
            \State $m \gets \mathcal{A}_S(m, B_t)$
        \EndFor
        
    \State \Return m
    \end{algorithmic}
    \end{algorithm}

    % , data influence model $\Theta$
