# Supplementary material for: Montessori-Instruct: Generate Influential Training Data Tailored for Student Learning
Source: arXiv:2410.14208 source file (2024-10-18)
Supplement: Supplementary file 2 [file cross_models.tex]

\begin{table}[h]
  \centering
    \scalebox{0.9}{
        \begin{tabular}{lccc}
        \toprule
        & \multicolumn{2}{c}{Alpaca Eval 2.0} & \multicolumn{1}{c}{MT-Bench}   \\
        \cmidrule(lr){2-3} \cmidrule(lr){4-4}
         Methods & LC-WR & WR & Overall \\  

        \midrule
        \textbf{\textit{Mistral-7B}} & & & \\
        pretrained model & 10.47\%& 14.92\%& 5.16\\
        $+$ \textit{self-instruct data} & 50\%& 50\%& 5.87\\
        $+$ \textit{dual-instruct data} &  52.92\%&  53.68\%& 6.13\\   
        
        \midrule
        \textbf{\textit{Qwen1.5-7B}} & & & \\
        pretrained model & 11.09\%& 17.25\%& 5.21\\
        $+$ \textit{self-instruct data} & 50\%& 50\%& 5.75\\
        $+$ \textit{dual-instruct data} &  53.82\%&  54.48\%& 5.87\\  
        
        \midrule
        \textbf{\textit{Gemma2-9B}} & & & \\
        pretrained model & 9.45\%& 14.62\%& 6.04\\
        $+$ \textit{self-instruct data} & 50\%& 50\%& 7.19\\
        $+$ \textit{dual-instruct data} &  52.58\%&  54.04\%&  7.74\\   
        \bottomrule
        \end{tabular}
    }
\caption{The data synthesized by our method can be used to different kinds of models}
% \vspace{-5mm} 
\label{tab:cross-models}
\end{table}
