# Supplementary material for: Montessori-Instruct: Generate Influential Training Data Tailored for Student Learning
Source: arXiv:2410.14208 source file (2024-10-18)
Supplement: Supplementary file 3 [file mt-bench-fine-grained.tex]

\begin{table}[h]
  \label{mt-bench-fine-grained}
  \centering
    \scalebox{0.74}{
        \begin{tabular}{lccccccccc}
        \toprule
        \multirow{2}{*}{Models} & \multicolumn{9}{c}{MT-Bench} \\
        \cmidrule(lr){2-10}  & Overall & Math & Coding & Extraction & STEM & Humanities & Writing & Roleplay & Reasoning \\
        \midrule
        pretrained model& 5.597& 1.9& 4.1& 4.85& 7.75& 7.95& 6.725& 6.8& 4.7\\
        \midrule
        \textbf{\textit{Self-Instruct}} & & & & & & & & & \\
 Llama3-8B-Instruct$_{\: teacher}$ & 6.49& 2.65 & 4.85 & 6.5 & 8.225 & 9.875 & 7.15 & 7.425 & 5.25\\
        gpt-4o$_{\: teacher} $ & 5.918& 3.55& 4.55& 7.85& 5.9& 6.9& 6.7& 7.05& 4.85\\
        \midrule
        \textbf{\textit{Self-reward}} & & & & & & & & & \\
        iter 1 & - & - & - & - & - & - & - & - & -\\
        iter 2 & - & - & - & - & - & - & - & - & -\\
        \midrule
        \textbf{\textit{LLM2LLM}} & & & & & & & & & \\
        iter 1 & 6.531& 3.09& 4.52& 7.92& 8.07& 9.982& 7.43& 6.97& 4.266\\
        iter 2 & 6.519& 3& 4.37& 7.17& 8.35& 10& 7.65& 6.96& 4.652\\
        \midrule
        \textit{\textbf{Ours}} & & & & & & & & &\\
        iter 1 & 6.825& 3.65 & 4.7 & 8.1 & 8.9 & 10.0 & 7.55 & 6.85 & 4.85\\
        iter 2 & 7.148& 4.65 & 4.6 & 7.58 & 9.225 & 9.7 & 8.95 & 7.7 & 4.8\\
        \bottomrule
        \end{tabular}
    }
\caption{Fine-grained MT-Bench of 8B models}
\end{table}

        % gpt-4o$_{\: teacher} $ & 5.597& 2.25 & 3.85 & 5.75 & 7.075 & 8.15 & 6.7 & 6.35 & 4.65\\
                % \midrule
        
 % llama3-8b-instruct(teacher)& 7.971& 5.45& 6.625& 8.0& 9.05& 9.9& 9.15& 9.15&6.45\\
